# Supplementary material for: Internal Calculi for Separation Logics
Source: arXiv:1910.05016 source file (2019-10-11)
Supplement: Supplementary file 1 [file appendix.tex]

\newpage
\section{A derivation in the proof system for \slSW}
\label{appendix-paragraphe-an-example}
\input{paragraph-an-example}

\section{Definition of the symbolic composition $\asymbunion$}
\label{appendix-definition-symbolic-composition}

\input{appendixproofs/definition-symbolic-composition}

 \cut{
\section{Proofs of Section~\ref{section:preliminaries}}

\subsection{Proof of Proposition~\ref{prop:sattoval}}

\begin{proof}(sketch)
  Let $\aformula$ be a formula having program variables from $\asetvar \subseteq_{\fin} \PVAR$, and let $\approx$ be an equivalence relation on $\asetvar$.
  The formula
  $\aformulabis_{\approx} \egdef (\emp \land \bigwedge_{\avariable \approx \avariablebis} \avariable = \avariablebis \land  \bigwedge_{\substack{\avariable \not\approx \avariablebis}} \avariable \neq \avariablebis )\implies (\aformula \septraction \true)$
  (parametric on $\approx$)
  can be shown to be valid if and only if
  for every store $\astore$ agreeing on $\approx$ there is a heap $\aheap$ such that $(\astore,\aheap) \models \aformula$.
  It is known
  %% (see~Lemma~1 of~\cite{Demri&Lozes&Mansutti18bis})
  that for  all stores $\astore,\astore'$ agreeing on $\approx$ and all heaps $\aheap$, the memory states $\pair{\astore}{\aheap}$ and $\pair{\astore'}{\aheap}$ satisfy the same set of formulae having variables from $\asetvar$.
  Then, since the antecedent of $\aformulabis_{\approx}$ is satisfiable, we conclude that $\aformulabis_{\approx}$ is valid if and only if there are a store $\astore$ agreeing on $\approx$ and a heap $\aheap$ such that $(\astore,\aheap) \models \aformula$.
  In order to check if $\aformula$ is satisfiable it is therefore sufficient to find an equivalence relation $\approx$ on $\asetvar$ such that $\aformulabis_{\approx}$ is valid. As the number of equivalence relations on $\asetvar$ is finite, we obtain a Turing reduction from satisfiability to validity.
\end{proof}
}

%% %REMOVE THIS FOR THE WHOLE APPENDIX
%% \end{document}

\ifLongVersionWithAppendix
\newpage
{\em Below, you will find the table of contents as well as technical appendices containing the proofs of the statements
from the body of the paper.
%% Initially, we did not expect that the proofs would be so lengthy but we have included it in the
%% document so that this can be read at the discretion of the reviewers.
It should also be noted that Appendix~\ref{appendix:DerivedTautologies} solely contains syntactic derivations in the calculus presented in Section~\ref{section:IntervalSL}, which are by nature lenghty.
}
\begin{flushright}
  \textbf{Appendices uploaded on \today.}
\end{flushright}

\tableofcontents

\section{Proofs of Section~\ref{section:PSL}}\label{appendix:Section3}

We recall that, given $\aliteral_1 \land \dots \land \aliteral_n \in \conjcomb{\coreformulae{\asetvar}{\bound}}$, we write $\literals{\aformula}$ to denote
$\{\aliteral_1,\dots,\aliteral_n\}$.
The notation $\aformulabis \inside \aformula$ is a shortcut for $\literals{\aformulabis} \subseteq \literals{\aformula}$.
Moreover, we write $\aformulater \inside \orliterals{\aformula}{\aformulabis}$ for
``$\aformulater \inside \aformula$ or $\aformulater \inside \aformulabis$'' and $\aformulater \inside \andliterals{\aformula}{\aformulabis}$ for ``$\aformulater \inside \aformula$ and $\aformulater \inside \aformulabis$''.
Similarly, $\orliterals{\aformula}{\aformulabis} \inside \aformulater$ (resp. $\andliterals{\aformula}{\aformulabis} \inside \aformulater$) stands for
``$\aformula \inside \aformulater$ or $\aformulabis \inside \aformulater$'' (resp. ``$\aformula \inside \aformulater$ and $\aformulabis \inside \aformulater$'').
Notice that the notation $\andliterals{\aformula}{\aformulabis} \inside \aformulater$ is not used nor defined in the body of the paper. However, it is (rarely) used in these appendices.

%% EL : uncomment if want to transfer the proof from core of the paper to the appendix
%% \subsection{Proof of Proposition~\ref{lemma:corePSLvalid}}
%% \lemmacorePSLvalid*
%% \begin{proof}
%% \input{appendixproofs/lemma-corePSLvalid}
%% \end{proof}

%% \subsection{Proof of Lemma~\ref{prop:corePSLone}}
%% \propcorePSLone*
%% \begin{proof}
%% \input{appendixproofs/property-corePSLone}
%% \end{proof}

%% \subsection{Proof of Lemma~\ref{prop:corePSLtwo}}
%% \propcorePSLtwo*
%% \begin{proof}
%% \input{appendixproofs/property-corePSLtwo}
%% \end{proof}

%% EL : a priori plus besoin de cette propriete
%% \subsection{Proof of Property~\ref{prop:corePSLthree}}
%% \propcorePSLthree*
%% \begin{proof}
%% \input{appendixproofs/property-corePSLthree}
%% \end{proof}

%% \subsection{Proof of Theorem~\ref{theo:corePSLcompl}}
%% \theocorePSLcompl*
%% \begin{proof}
%% \input{appendixproofs/theo-corePSLcompl}
%% \end{proof}

%% \subsection{Proof of Lemma~\ref{lemma:starPSLvalid}}
%% \lemmastarPSLvalid*
%% \begin{proof}
%% \input{appendixproofs/lemma-starPSLvalid}
%% \end{proof}

\subsection{Proof of Lemma~\ref{prop:corePSLtwo}}
\input{appendixproofs/proof-corePSLtwo}

\subsection{Proof of Theorem~\ref{theo:corePSLcompl}}
\input{appendixproofs/proof-theorem-corePSLcompl}

\subsection{Proof of Proposition~\ref{prop:admissible-axioms-1}}
\label{appendix-proof-proposition-admissible-axioms-1}

%% \propadmissibleaxiomsone*

\begin{restatable}{proposition}{propadmissibleaxiomsone}\label{prop:admissible-axioms-1}
Axioms $\ref{coreAx:Size}$ and $\ref{coreAx:AllocSize}$ are derivable
in $\coresys(*)$.
\end{restatable}

\begin{proof}
\input{appendixproofs/proposition-admissible-axioms-1}
\end{proof}

\subsection{Proof of Lemma~\ref{lemma:starPSLelim}}
\lemmastarPSLelim*
\begin{proof}
\input{appendixproofs/lemma-starPSLelim}
\end{proof}

\subsection{Proof of Theorem~\ref{theo:starCompleteness}}
\theostarCompleteness*

\begin{proof}
\input{appendixproofs/theo-starPSLelim}
\end{proof}

\subsection{Proof of Soundness of $\coresys(\separate,\magicwand)$}\label{appendix:PSLSoundness}
We prove Lemma~\ref{lemma:magicwandPSLvalid}.
By showing Lemma~\ref{lemma:magicwandPSLvalid}, we also show
soundness of the restriction of the proof system.
%% Propositions~\ref{lemma:corePSLvalid} and~\ref{lemma:starPSLvalid}.

\begin{restatable}{lemma}{lemmamagicwandPSLvalid}\label{lemma:magicwandPSLvalid}
$\magicwandsys$ is sound.
\end{restatable}
\begin{proof}
\input{appendixproofs/lemma-PSLvalid}
\end{proof}

\subsection{Proof of Proposition~\ref{prop:admissible-axioms-2}}
\label{appendix-proposition-admissible-axioms-2}
%% \propadmissibleaxiomstwo*

\begin{restatable}{proposition}{propadmissibleaxiomstwo}\label{prop:admissible-axioms-2}
The axioms~\ref{starAx:DistrOr},~\ref{starAx:False},~\ref{starAx:StarAlloc} and~\ref{starAx:DoubleAlloc} are derivable
in $\coresys(\separate,\magicwand)$.
\end{restatable}

\begin{proof}
\input{appendixproofs/proposition-admissible-axioms-2}
\end{proof}

%% \subsection{Proof of Lemma~\ref{lemma:septractioncongruence}}
%% \lemmaseptractioncongruence*
%%

\subsection{Proof of Lemma~\ref{lemma:magicwandPSLelim}}
\label{appendix-proof-lemma-magicwandPSLelim}

\input{appendixproofs/lemma-magicwandPSLelim}

%% \subsection{Proof of Theorem~\ref{theo:magicwandPSLelim}}
%% \theomagicwandPSLelim*
%% \begin{proof}
%% \input{appendixproofs/theo-magicwandPSLelim}
%% \end{proof}

 \subsection{Proof of Theorem~\ref{theo:PSLcompleteAx}}
 \theoPSLcompleteAx*
 \begin{proof}
 \input{appendixproofs/theo-PSLcompleteAx}
 \end{proof}

\newpage
\section{Proofs of Section~\ref{section:IntervalSL}}\label{appendix:Section4}

First, we need to introduce preliminary definitions. Given an arbitrary object $\mathtt{O}$ (for instance, this can be a term
in $\atermset{\PVAR}$, a set of terms --or of pairs of terms--), we write $\chars{\mathtt{O}}$ to denote the set of program
variables occurring in $\mathtt{O}$. For instance, by definition,
$\chars{\ameetvar{\avariable}{\avariablebis}{\avariableter}} = \{\avariable,\avariablebis,\avariableter\}$.
By contrast, we write $\vars{\mathtt{O}}$ to denote the subset of $\chars{\mathtt{O}}$ made of the program variables
occurring in $\mathtt{O}$ truncated by all the meet-point terms. For instance, by definition,
$\vars{\set{\avariableter, \ameetvar{\avariable}{\avariablebis}{\avariableter}}} = \set{\avariableter}$.
Similarly, we write $\meets{\mathtt{O}}$ to denote the set of meet-point terms  occurring in $\mathtt{O}$.
For example, by definition, $\meets{\set{\avariableter, \ameetvar{\avariable}{\avariablebis}{\avariableter}}} =
\set{\ameetvar{\avariable}{\avariablebis}{\avariableter}}$.
Some of these definitions are already provided in the body of the paper (see e.g. Section~\ref{section-exists-elimination}).

\input{appendixproofs/intervalSL-auxiliary-lemmata-and-proofs}

%% \subsection{Expressing core formulae in \intervalSL}
\subsection{Proof of Lemma~\ref{lemma:coreIntCoreExpress}}\label{appendix:ExpressingCoreFormulae}
\input{appendixproofs/proof-lemmaintcoreexpress}

\subsection{Proof of Lemma~\ref{lemma:axiomstwocoresound}}

\lemmaaxiomstwocoresound*

\input{appendixproofs/proof-lemma-axiomstwosound}

\subsection{Abstract memory states and proof of Lemma~\ref{lemma:msmodelsabs}}
\input{appendixproofs/proof-lemma-ms-models-abs}

\subsection{Proof of Lemma~\ref{lemma:axiomtwoRCct}}
%%
%% SD 27/06/2019: to be uniform in the way we have section titles
%%
%%  ($\coresys$ is complete for characteristic formulae)

\input{appendixproofs/proof-lemma-axiomstwo-RCchar}

\subsubsection{Equivalence (in $\coresys$) between core types and characteristic formulae}
\input{appendixproofs/proof-lemmacoretypecharsms}

\subsubsection{Completeness of $\coresys$ for core types (Lemma~\ref{lemma:axiomtwoRCct})}
\input{appendixproofs/proof-lemmaaxiomtwoRCct}

\subsection{Proof of Theorem~\ref{theo:core2PSLcompl}}

\theocoretwoPSLcompl*

\input{appendixproofs/proof-theo-core2PSLcompl}

\subsection{Soundness of $\coresys(\weirdexists)$}\label{appendix-ExistsSoundness}
\input{appendixproofs/proof-lemma-exists-axioms-valid}

\subsection{Proof of Lemma~\ref{lemma:axiomseliminateexists}}\label{appendix-eliminate-exists}
\input{appendixproofs/proof-lemma-axioms-eliminate-exists}

\subsection{Results on the composition of symbolic memory states}\label{appendix:CompositionMemoryState}
\input{appendixproofs/proofs-composition-sms}

\subsection{Soundness of $\coresys(\separate,\weirdexists)$}\label{appendix-StarSoundness}
\input{appendixproofs/proof-lemma-axiomtwo-StarSound}

\subsection{Constructive elimination of separating conjunction $\separate$}
\label{appendix-starelimination}

\input{appendixproofs/proof-lemma-axiomtwo-StarElimination}

\subsection{Proof of Theorem~\ref{theo:axioms2soundcomplete}}

\theoaxiomstwosoundcomplete*

\input{appendixproofs/proof-theoremaxioms2soundcomplete}

\subsection{Proof of Theorem~\ref{theorem:pspace}}
\input{appendixproofs/proof-pspace}

%%%%%%%%%%%%%%%%%%%%%%%%%%%%%%%%%%%%%%%%%%%%%%%%%%%%%%%%%%%%%%%%%%%%%%%%%%%%%%%
%%%LEAVE THIS SUBSECTION AT THE END
%%%%%%%%%%%%%%%%%%%%%%%%%%%%%%%%%%%%%%%%%%%%%%%%%%%%%%%%%%%%%%%%%%%%%%%%%%%%%%%
\newpage
\section{Derived tautologies used in the proofs of Section~\ref{section:IntervalSL}}\label{appendix:DerivedTautologies}
First, we recall the list of shorthands used to state the axioms and that are used in what follows.
Let $\pair{\astore}{\aheap}$ be a memory state.
We introduce the formula $\defined{\ameetvar{\avariable}{\avariablebis}{\avariableter}}$, satisfied if and only if $\semantics{\ameetvar{\avariable}{\avariablebis}{\avariableter}}_{\astore,\aheap}$ is defined.
Similarly, we introduce the formula $\symmetric{\ameetvar{\avariable}{\avariablebis}{\avariableter}}$ (resp. $\asymmetric{\ameetvar{\avariable}{\avariablebis}{\avariableter}}$) that refine the notion of $\defined{\ameetvar{\avariable}{\avariablebis}{\avariableter}}$
by also requiring that $\semantics{\ameetvar{\avariable}{\avariablebis}{\avariableter}}_{\astore,\aheap} = \semantics{\ameetvar{\avariablebis}{\avariable}{\avariableter}}_{\astore,\aheap}$
(resp.  $\semantics{\ameetvar{\avariable}{\avariablebis}{\avariableter}}_{\astore,\aheap} \neq \semantics{\ameetvar{\avariablebis}{\avariable}{\avariableter}}_{\astore,\aheap}$).
These formulae, that are trivially extended to variable, are defined as follows.
\begin{itemize}
\begin{minipage}{0.3\linewidth}
\item $\defined{\avariable} \egdef \true$
\item $\symmetric{\avariable} \egdef \true$
\item $\asymmetric{\avariable} \egdef \false$
\end{minipage}
\begin{minipage}{0.7\linewidth}
\item $\defined{\ameetvar{\avariable}{\avariablebis}{\avariableter}} \egdef \ameetvar{\avariable}{\avariablebis}{\avariableter} = \ameetvar{\avariable}{\avariablebis}{\avariableter}$
\item $\symmetric{\ameetvar{\avariable}{\avariablebis}{\avariableter}} \egdef \ameetvar{\avariable}{\avariablebis}{\avariableter} = \ameetvar{\avariablebis}{\avariable}{\avariableter}$
\item $\asymmetric{\ameetvar{\avariable}{\avariablebis}{\avariableter}} \egdef \defined{\ameetvar{\avariable}{\avariablebis}{\avariableter}} \land \lnot \symmetric{\ameetvar{\avariable}{\avariablebis}{\avariableter}}$
\end{minipage}
\end{itemize}
We introduce the formula $\before{\aterm}{\aterm'}$, satisfying the following property:
\begin{nscenter}
$\pair{\astore}{\aheap} \models \before{\aterm}{\aterm'}$ iff
$\begin{aligned}[t]
&\semantics{\aterm}_{\astore,\aheap} \neq \semantics{\aterm'}_{\astore,\aheap},\ \minpath{\semantics{\aterm}_{\astore,\aheap}}{\semantics{\aterm'}_{\astore,\aheap}}{\aheap} \neq \emptyset\ \text{and}\\
&\text{every location}\ \alocation \in \minpath{\semantics{\aterm}_{\astore,\aheap}}{\semantics{\aterm'}_{\astore,\aheap}}{\aheap}\
\text{is not in a cycle.}
\end{aligned}$
\end{nscenter}
It is defined as follows:
\begin{itemize}
\item $\before{\ameetvar{\avariable}{\avariablebis}{\avariableter}}{\ameetvar{\avariable}{\avariablefour}{\avariablefifth}}$ is defined as
\begin{nscenter}
$
  \symmetric{\ameetvar{\avariable}{\avariablebis}{\avariableter}} \land \defined{\ameetvar{\avariable}{\avariablebis}{\avariablefifth}}
  \land \defined{\ameetvar{\avariable}{\avariablefour}{\avariablefifth}}
  \land \ameetvar{\avariable}{\avariablebis}{\avariableter} \neq \ameetvar{\avariable}{\avariablefour}{\avariablefifth}
  \land \ameetvar{\avariable}{\avariablebis}{\avariableter} \neq \ameetvar{\avariablebis}{\avariablefour}{\avariablefifth}
$
\end{nscenter}
\item $\before{\ameetvar{\avariablebis}{\avariable}{\avariableter}}{\ameetvar{\avariable}{\avariablefour}{\avariablefifth}} \egdef
\before{\ameetvar{\avariable}{\avariablebis}{\avariableter}}{\ameetvar{\avariable}{\avariablefour}{\avariablefifth}}$
\item $
\before{\ameetvar{\avariable}{\avariablebis}{\avariableter}}{\ameetvar{\avariablefour}{\avariablefifth}{\avariablesix}} \egdef
  \bigvee_{a \in \{\avariablefour,\avariablefifth\}} \before{\ameetvar{\avariable}{\avariablebis}{\avariableter}}{\ameetvar{\avariable}{a}{\avariablesix}} \land
    \ameetvar{\avariable}{a}{\avariablesix} = \ameetvar{\avariablefour}{\avariablefifth}{\avariablesix}
$
\item $\before{\avariable}{\aterm} \egdef \before{\ameetvar{\avariable}{\avariable}{\avariable}}{\aterm}$
\item $\before{\aterm}{\avariable} \egdef \before{\aterm}{\ameetvar{\avariable}{\avariable}{\avariable}}$
\end{itemize}
We introduce the formula $\sameloop{\aterm}{\aterm'}$, satisfying the following property:
\begin{nscenter}
$\pair{\astore}{\aheap} \models \sameloop{\aterm}{\aterm'}$ iff
$\begin{aligned}[t]
&\semantics{\aterm}_{\astore,\aheap} \neq \semantics{\aterm'}_{\astore,\aheap}\ \text{and}\\
&\minpath{\semantics{\aterm}_{\astore,\aheap}}{\semantics{\aterm}_{\astore,\aheap}}{\aheap} = \minpath{\semantics{\aterm'}_{\astore,\aheap}}{\semantics{\aterm'}_{\astore,\aheap}}{\aheap} \neq \emptyset
\end{aligned}$
\end{nscenter}
It is defined as follows:
\begin{itemize}
\item $\sameloop{\ameetvar{\avariable}{\avariablebis}{\avariableter}}{\ameetvar{\avariablefour}{\avariablefifth}{\avariablesix}} \egdef
\ameetvar{\avariable}{\avariablebis}{\avariableter} = \ameetvar{\avariable}{\avariablefour}{\avariablesix} \land \ameetvar{\avariablefour}{\avariablefifth}{\avariablesix} = \ameetvar{\avariablefour}{\avariable}{\avariableter} \land \asymmetric{\ameetvar{\avariable}{\avariablefour}{\avariableter}}$
\item $\sameloop{\avariable}{\aterm} \egdef \sameloop{\ameetvar{\avariable}{\avariable}{\avariable}}{\aterm}$
\item $\sameloop{\aterm}{\avariable} \egdef \sameloop{\avariable}{\aterm}$
\end{itemize}
We now provide a list of valid formulae.
These forulae are derivable tautologies in the axiom system and are helpful to ease the proof of Lemma~\ref{lemma:axiomstwoRCchars} and Lemma~\ref{lemma:coretypecharsms}.
The proofs of such formulae are all given in the style of Fitch proofs, as introduced in the beginning of Appendix~\ref{appendix:Section4}.

Recall that we use the following notations for tautologies of propositional calculus:

\begin{tabular}{lcl}
\landcontr & : & $\aformula \land \lnot \aformula \implies \bottom$\\
\landtwo & : & $\aformula \implies \aformula \land \aformula$\\
\modusponens & : & $(\aformula \implies \aformulabis) \land \aformula \implies \aformulabis$\\
$\lor\text{I}$ & : & $\aformula \implies \aformula \lor \aformulabis$\\
$\land\text{E}$ & : & $\aformula_1 \land \aformula_2 \land \dots \land \aformula_n \implies \aformulabis_1 \land \aformulabis_2 \land \dots \land \aformulabis_m$, where $\{\aformulabis_1,\dots,\aformulabis_n\}\subseteq\{\aformula_1,\dots,\aformula_m\}$
\\
\lorimpL & : & $(\aformula \lor \aformulabis) \land (\aformula \implies \aformulater) \implies \aformulater \lor \aformulabis$\\
\lorimpR & : & $(\aformula \lor \aformulabis) \land (\aformulabis \implies \aformulater) \implies (\aformula \lor \aformulater)$\\
$\lor\text{E}$ & : & $(\Gamma \Rightarrow ((\aformula \lor \aformulabis) \land (\aformula \Rightarrow \aformulater)\land(\aformulabis \Rightarrow \aformulater))) \implies (\Gamma \Rightarrow \aformulater)$\qquad (proof by cases)
\\
$\lnot\text{I}$ & : & $(\Gamma \Rightarrow (\aformula \Rightarrow \bottom)) \implies (\Gamma \Rightarrow \lnot \aformula)$\qquad (proof ad absurdum)
\end{tabular}

\begin{adjustwidth}{-3cm}{-3cm}
\begin{multicols}{2}
\relscale{0.8}
\nolinenumbers

\subsection{Intermediate tautologies about equalities}
\label{subsection-intermediate-tautologies-eq}
\input{appendixproofs/apdxsection-int-taut-eq}

\subsection{Intermediate tautologies about $\mathtt{sees}$}
\label{subsection-intermediate-tautologies-sees}
\input{appendixproofs/apdxsection-int-taut-sees}

\end{multicols}
\end{adjustwidth}
\fi
